# Supplementary material for: Carbon-Intelligent Global Routing in Path-Aware Networks
Source: arXiv:2211.00347 source file (2023-05-01)
Supplement: Supplementary file 1 [file electricity-cost-estimate.tex]

\section{Estimating Electricity Price
for Different Sources}
\label{apdx:electricity-price}

Importantly, ISPs are themselves consumers
in the electricity market. Hence, the 
relevant electricity cost metric for ISPs
is not the generation cost of electricity,
but the retail price (including profit 
margins, taxes and fees). However,
to the best of our knowledge,
retail-price data for different sources
of electricity generation across countries 
is not readily available.
We therefore estimate the retail-price
difference between low-emission and 
high-emission electricity on the basis of both
generation costs and integration costs.

Regarding the generation cost of
electricity, we rely on the
well-established 
\emph{levelized cost of energy (LCOE)},
which allows a limited comparison of
electricity-generation sources with
different cost structures. The basic
idea of the LCOE metric is to divide
the total cost accumulating over the
life cycle of an electricity-generating
system (investment, operation, maintenance,
fuel and decommissioning expenditures)
by its generated electricity
volume, while taking into account
capital costs and discount 
rates~\cite{ueckerdt2013system}.
LCOE estimates depend on the exact
methodology, assumptions and paremeters
used in the analysis. Hence, we
rely on LCOE estimates from multiple
studies, namely the following three:
\begin{itemize}
    \item \textbf{Lazard's Levelized Cost of Energy Analysis - Version 14.0 (2020) \cite{lazard2020levelized}:} This study
    claims global validity and presents
    LCOE estimates in USD/MWh.
    \item \textbf{LCOE Estimates for Renewable Energy by Fraunhofer Institute of Solar Energy Systems (F-ISE, 2018) \cite{kost2018levelized}:} This study
    is based on an analysis of the German
    energy system and presents LCOE estimates
    in EUR/MWh, which have been converted
    with an exchange rate of 1.21 USD/EUR.
    \item \textbf{LCOE Estimates by the Paul Scherrer Institute (PSI, 2017) \cite{bauer2017potentials}:} This study
    is based on an analysis of the Swiss
    energy system (accounting for imports)
    and presents LCOE estimates in CHF/MWh,
    which roughly correspond to LCOE estimates
    in USD/MWh because of long-term parity
    between CHF and USD. While the study
    was published in 2017, it contains
    LCOE predictions for 2020.
\end{itemize}

While LCOE is a helpful basis for
comparison, this metric is not sufficient.
As noted by Joskow~\cite{joskow2011comparing}
and Ueckerdt et al.~\cite{ueckerdt2013system},
the LCOE metric only allows a comparison
of electricity-generating technologies
with respect to their cost, but ignores
the differences in value between different
forms of electricity production. In
particular, variable renewable
energies (VRE), including wind and solar,
have a lower value than conventionally
generated electricity due to their
variability and remote production.
If VRE are integrated into an energy
system, they incur balancing costs
(backup production capacity 
needed to absorb shortfalls from
prediction errors), grid-related
costs (grid upgrades needed to transfer
electricity from remote centers of
VRE production to consumption centers),
and profile costs (inefficiency arising
from discrepancy between production
peaks and consumption 
peaks)~\cite{hirth2015integration}.
These costs depend on the
extent of VRE penetration, as higher
penetration leads to higher variability
and a smaller residual energy system
usable for back-up.
In a meta-review of over 100 studies,
Hirth et al.~\cite{hirth2015integration}
estimate that these different variants
of integration costs sum up to additional
costs of around
30--42 USD/MWh for wind power at a
wind penetration of 30-40\%, while
conventional plants have negligible
integration costs. We assume that
these integration costs are also
valid for solar-based electricity
production. These integration
costs have been added to the analysis
in Table~\ref{tab:lcoe}.

The LCOE overview presented in 
Table~\ref{tab:lcoe}
illustrates that LCOE estimates
vary considerably between studies,
which is due to different
methodologies, geographical contexts,
and publication dates of the studies.
As it is difficult to compare
individual LCOE estimates of
different studies due to differences
in methodology, we calculate
the cost penalty of low-emission
sources of electricity generation
over high-emission sources for
each study separately.
The average of these cost penalties,
which are comparable across studies,
is 1.34, meaning that electricity generation
from low-emission sources is 34\%
more expensive than from high-emission sources.
\begin{table*}[t!]
    \centering
    \caption{Levelized cost of energy (LCOE) for
    different technologies of electricity generation in USD/MWh. LCOE of variable renewable energy (VRE) technologies (solar and wind) are
    extended with integration costs
    according to an estimate by Hirth
    et al.~\cite{hirth2015integration}.}
    \begin{tabular}{c|c|c|c|c}
        \multicolumn{2}{c|}{} & \multicolumn{3}{c}{Study}\\
        \cline{3-5}
        \multicolumn{2}{c|}{Electricity source} & Lazard~\cite{lazard2020levelized} 
        & F-ISE~\cite{kost2018levelized}
        & PSI~\cite{bauer2017potentials}\\
        \toprule \multirow{11}{*}{\textbf{Low-emission}} & Solar (utility) & 
        29 -- 42 & 45 -- 140  & 90 -- 110\\
        \cline{2-5} & \textit{with integration costs}
        & 59 -- 84 & 75 -- 182 & 120 -- 152\\
        \cline{2-5}  & Wind (onshore) &
        26 -- 54 & 48 -- 100 & 40 -- 190\\
        \cline{2-5}  & \textit{with integration costs} &
        56 -- 96 & 78 -- 142 & 70 -- 232\\
        \cline{2-5}  & Wind (offshore) & 86 & 91 -- 167 & 130 -- 250 \\
        \cline{2-5}  & \textit{with integration costs} &
        116 -- 128 & 121 -- 209 & 160 -- 292\\
        \cline{2-5}  & Hydro (large, new) & -- & -- & 141\\
        \cline{2-5} & Hydro (large, amortized) & -- & -- & 50 -- 80\\
        \cline{2-5} & Nuclear (new) & 129 -- 198 & -- & 51 -- 124\\
        \cline{2-5}  & Nuclear (amortized) & 29 & -- & 40 -- 60\\
        \cmidrule{2-5} & \makecell{Average (equally weighted, all)} & 77 & 135 & 122\\
        \midrule \multirow{5}{*}{\textbf{High-emission}} & Coal (new) & 65 -- 159 & 56 -- 119 & 41 -- 84\\
        \cline{2-5} & Coal (amortized) & 41 & -- & --\\
        \cline{2-5} & Gas CC (new) & 44 -- 73 & 94 -- 121 & 111 -- 126\\
        \cline{2-5} & Gas CC (amortized) & 28 & -- & -- \\
        \cmidrule{2-5} & Average (equally weighted, all) & 60 & 98 & 90\\
        \midrule \multicolumn{2}{c|}{\makecell{Generation-cost penalty of low-emission sources\\
        over high-emission sources}} & 1.28 & 1.38 & 1.36\\
        \hline \multicolumn{2}{c|}{\textbf{Average generation-cost penalty}}
        & \multicolumn{3}{c}{1.34}
    \end{tabular}
    \label{tab:lcoe}
\end{table*}  However, as mentioned initially,
the relevant electricity cost for ISPs
is not the generation cost for
electricity providers, but the retail
price charged by these providers.
Since this retail price includes
a considerable technology-independent 
fixed component in addition to the
generation cost, the increase in retail
price for low-emission electricity
should be lower than the corresponding increase
in generation cost.

In order to estimate the non-generation
price component (NGPC) of 
electricity retail prices,
we perform the analysis in
Table~\ref{tab:retail-price}.
In this analysis, we calculate the
average generation cost for
an MWh in the European Union
according to the composition of
the EU electricity sector, 
compare it to the average retail price
per MWh that is charged to
non-household end consumers and 
consider the difference
the NGPC. The result of this
analysis is that a MWh in
the European Union has
an average generation cost 
of around 80 USD, a retail price
of around 180 USD and thus
an average NGPC of around 
100 USD. Hence, generation cost
makes up only 44\% of the
end-consumer price, which
is consistent with another
estimate~\cite{murray2019paradox}.

Finally, we estimate the difference
in electricity retail price 
between low-emission electricity 
and high-emission electricity.
Using the augmented Lazard
estimates (cf. Table~\ref{tab:lcoe})
for generation costs of 77 USD/MWh
and 60 USD/MWh for low-emission
and high-emission electricity, respectively,
we arrive at the following price
ratio assuming a NGPC of 100 USD/MWh:
\begin{equation}
    \frac{77 + 100}{60 + 100} = \frac{177}{160} \approx 1.1
\end{equation}
In the following, we will thus assume
that switching to low-emission electricity
will increase the energy costs of
an ISP by 10\%.
\begin{table*}[t!]
    \centering
    \caption{Estimate of non-generation
    price component (NGPC) in electricity retail prices
    in EU countries in 2019. All cost and
    price values are in USD/MWh. The LCOE values
    for generation cost of different
    technologies are from the Lazard study~\cite{lazard2020levelized}
    (except the hydro LCOE, which is from
    the PSI study~\cite{bauer2017potentials}),
    and include integration costs.
    The data on the composition
    of EU electricity production are from the European Commission~\cite{ec2020generation}
    and the International Energy Agency~\cite{iea2020eugeneration}.
    The retail-price data refer to
    non-household consumers in the European Union~\cite{ec2020prices},
    include all taxes and levies and
    have been converted to USD with
    an exchange rate of 1.21 USD/EUR.}
    \begin{tabular}{c|c|c|c|c|c}
        \makecell{Electricity\\source} & \makecell{LCOE\\(avg)} & \makecell{Share of EU\\
        electricity\\production} & \makecell{Generation cost\\(avg MWh)} & \makecell{
        Retail price\\(avg)} & \makecell{NGPC}\\
        \toprule Solar & 72 & 4.4 & \multirow{6}{*}{80} & \multirow{6}{*}{180} & \multirow{6}{*}{100}\\
        \cline{1-3} Wind & 100 & 13.3 & &\\
        \cline{1-3} Hydro & 103 & 12.3 & &\\
        \cline{1-3} Nuclear & 94 & 26.7 & &\\
        \cline{1-3} Coal & 77 & 21.4 & &\\
        \cline{1-3} Gas & 43 & 21.4 & &\\
    \end{tabular}
    \label{tab:retail-price}
\end{table*}
