# Supplementary material for: Carbon-Intelligent Global Routing in Path-Aware Networks
Source: arXiv:2211.00347 source file (2023-05-01)
Supplement: Supplementary file 2 [file impact_on_latency.tex]

\section{Extended discussion: impacts on the network}\label{apdx:impact_on_quality}
 \paragraph{Convergence of the virtuous feedback cycle} \cref{fig:economic-simulation:correlation} (cf.~\Cref{sec:eval_virtuous})
 highlights that the introduction of
 carbon awareness into path discovery
 and path selection leads to a
 \emph{virtuous cycle}: By improving
 their carbon footprint, ISPs can attract
 additional traffic and thereby increase
 their profit. As a result, the offered
 paths become increasingly carbon-neutral: 
 Over the simulation duration, the average green-energy 
 share grows by 6 percentage points,
 the total emissions are reduced by 20\%,
 and the average carbon intensity of forwarding
 is reduced by 13\%. In general, this decarbonization
 process also leads to higher prices for end-host
 service and inter-AS links as the ISPs shift
 their higher energy costs to their customers.
 Because of traffic elasticity 
 (cf.~\cref{eq:market:demand:path}),
 this higher price level causes a slight drop
 in the total traffic volume that is actually
 sent, which explains the difference 
 between the reductions in total
 emissions and carbon intensity. 
 Eventually, the decarbonization process
 should converge when the cost for
 additional green-energy purchases exceeds
 the revenue from additional traffic
 that can be attracted through carbon-footprint
 improvements; however, this convergence point is 
 not reached within the duration of our simulation.
